# Supplementary material for: Improved Conditional VRNNs for Video Prediction
Source: arXiv:1904.12165 source file (2019-04-27)
Supplement: Supplementary file 1 [file appendix.tex]

\appendix
\counterwithin{figure}{section}
\onecolumn

{
\hfill\large\bfseries Supplementary Material: Improved Conditional VRNNs for Video Prediction\hfill
}

\section{Hierarchical VRNN}

\subsection{ELBO Derivation}

We start from the ELBO for VRNNs ~\cite{vrnn}:

\begin{equation}
    \log p(\mathbf{x}|\mathbf{c}) \ge \sum_{t=1}^T \mathbb{E}_{q({z_{t}}|\mathbf{z_{<t}}, \mathbf{x_{\leq t}}, \mathbf{c})}\log p(x_t | \mathbf{z_{\leq t}}, \mathbf{x_{< t}}, \mathbf{c}) - D_{KL}(q(z_t|\mathbf{z_{<t}}, \mathbf{x_{\leq t}}, \mathbf{c}) || p(z_t| \mathbf{z_{<t}}, \mathbf{x_{< t}}, \mathbf{c}))
\end{equation}

Recall we defined $\mathbf{z_t}=({z^1_t}, ..., {z^L_t})$ and factorized the prior as:

\begin{equation}
p(\mathbf{z_t}| \mathbf{z_{<t}}, \mathbf{x_{<t}}, \mathbf{c}) = \prod_{l=1}^L p(z_t^l| \mathbf{z_{t}^{<l}}, \mathbf{z_{<t}^{l}}, \mathbf{x_{<t}}, \mathbf{c}).
\end{equation}

And the posterior:
\begin{equation}
q(\mathbf{\mathbf{z_t}}|\mathbf{z_{<t}}, \mathbf{x_{\leq t}}, \mathbf{c}) = \prod_{l=1}^L q(z_t^l| \mathbf{z_{t}^{<l}}, \mathbf{z_{<t}^{l}}, \mathbf{x_{ \leq t}}, \mathbf{c}).
\end{equation}

We then substitute these terms in the VRNN ELBO, first looking at the reconstruction term inside the summation over time:
\begin{align}
\begin{split}
    \sum^{T}_{t=1}\mathbb{E}_{q(\mathbf{z_{t}}|\mathbf{z_{<t}}, \mathbf{x_{\leq t}}, \mathbf{c})}\log p(x_t | \mathbf{z_{\leq t}}, \mathbf{x_{< t}}, \mathbf{c}) 
    & = 
    \sum^{T}_{t=1}\mathbb{E}_{q(z^{1}_{t}, ..., z^{L}_{t}|\mathbf{z_{<t}}, \mathbf{x_{\leq t}}, \mathbf{c})} \log p(x_t | z^{1}_{t}, ..., z^{L}_{t}, \mathbf{z_{< t}}, \mathbf{x_{< t}}, \mathbf{c})  \\
    & =
    \sum^{T}_{t=1}\mathbb{E}_{q(z^{1}_{t}|\mathbf{z_{<t}}, \mathbf{x_{\leq t}}, \mathbf{c}) ... q(z^{L}_{t}|\mathbf{z^{<L}_t}, \mathbf{z_{<t}}, \mathbf{x_{\leq t}}, \mathbf{c})} \log p(x_t | z^{1}_{t}, ..., z^{L}_{t}, \mathbf{z_{< t}}, \mathbf{x_{< t}}, \mathbf{c}) 
\end{split}
\end{align}

And then looking at the summation of KL divergences:
\begin{align}
\begin{split}
    -\sum^{T}_{t=1}\mathbb{E}_{q(\mathbf{z_{t}}|\mathbf{z_{<t}}, \mathbf{x_{\leq t}}, \mathbf{c})} & \log 
    \frac{q(\mathbf{z_{t}}|\mathbf{z_{<t}}, \mathbf{x_{\leq t}}, \mathbf{c})}{p(\mathbf{z_{t}}|\mathbf{z_{<t}}, \mathbf{x_{< t}}, \mathbf{c})}
    = 
    -\sum^{T}_{t=1}\mathbb{E}_{q(z^{1}_{t}, ..., z^{L}_{t}|\mathbf{z_{<t}}, \mathbf{x_{\leq t}}, \mathbf{c})}\log 
    \frac{q(z^{1}_{t}, ..., z^{L}_{t}|\mathbf{z_{<t}}, \mathbf{x_{\leq t}}, \mathbf{c})}{p(z^{1}_{t}, ..., z^{L}_{t}|\mathbf{z_{<t}}, \mathbf{x_{< t}}, \mathbf{c})}
    \\ & =
    -\sum^{T}_{t=1}\mathbb{E}_{q(z^{1}_{t}|\mathbf{z_{<t}}, \mathbf{x_{\leq t}}, \mathbf{c}) ... q(z^{L}_{t}|\mathbf{z^{<L}_t}, \mathbf{z_{<t}}, \mathbf{x_{\leq t}}, \mathbf{c})}\log 
    \frac{q(z^{1}_{t}|\mathbf{z_{<t}}, \mathbf{x_{\leq t}}, \mathbf{c}) ... q(z^{L}_{t}|\mathbf{z^{<L}_t}, \mathbf{z_{<t}}, \mathbf{x_{\leq t}})}{p(z^{1}_{t}|\mathbf{z_{<t}}, \mathbf{x_{\leq t}}, \mathbf{c}) ... q(z^{L}_{t}|\mathbf{z^{<L}_t}, \mathbf{z_{<t}}, \mathbf{x_{< t}})}
     \\ & =
    -\sum^{T}_{t=1}\mathbb{E}_{q(z^{1}_{t}|\mathbf{z_{<t}}, \mathbf{x_{\leq t}}, \mathbf{c}) ... q(z^{L}_{t}|\mathbf{z^{<L}_t}, \mathbf{z_{<t}}, \mathbf{x_{\leq t}}, \mathbf{c})}\log 
    \frac{q(z^{1}_{t}|\mathbf{z_{<t}}, \mathbf{x_{\leq t}}, \mathbf{c}) ... q(z^{L}_{t}|\mathbf{z^{<L}_t}, \mathbf{z_{<t}}, \mathbf{x_{\leq t}})}{p(z^{1}_{t}|\mathbf{z_{<t}}, \mathbf{x_{\leq t}}, \mathbf{c}) ... q(z^{L}_{t}|\mathbf{z^{<L}_t}, \mathbf{z_{<t}}, \mathbf{x_{< t}})}
    \\ 
    & \text{(by definition of conditional KL divergence)}
    \\ & = 
    -\sum^{T}_{t=1}\sum^{L}_{l=1} D_{KL}((q(z_t|\mathbf{z_{<t}}, \mathbf{x_{\leq t}}, \mathbf{c}) || p(z_t| \mathbf{z_{<t}}, \mathbf{x_{< t}}, \mathbf{c}))
\end{split}
\end{align}

Adding both terms together we obtain the ELBO defined in eq.~\ref{eq:hier_elbo}.

\subsection{Posterior Dense Connectivity}
\label{app:posterior_dense}
\begin{figure}[t]
 \begin{center}
    \includegraphics[trim=10 68 10 27, clip,width=0.45\textwidth]{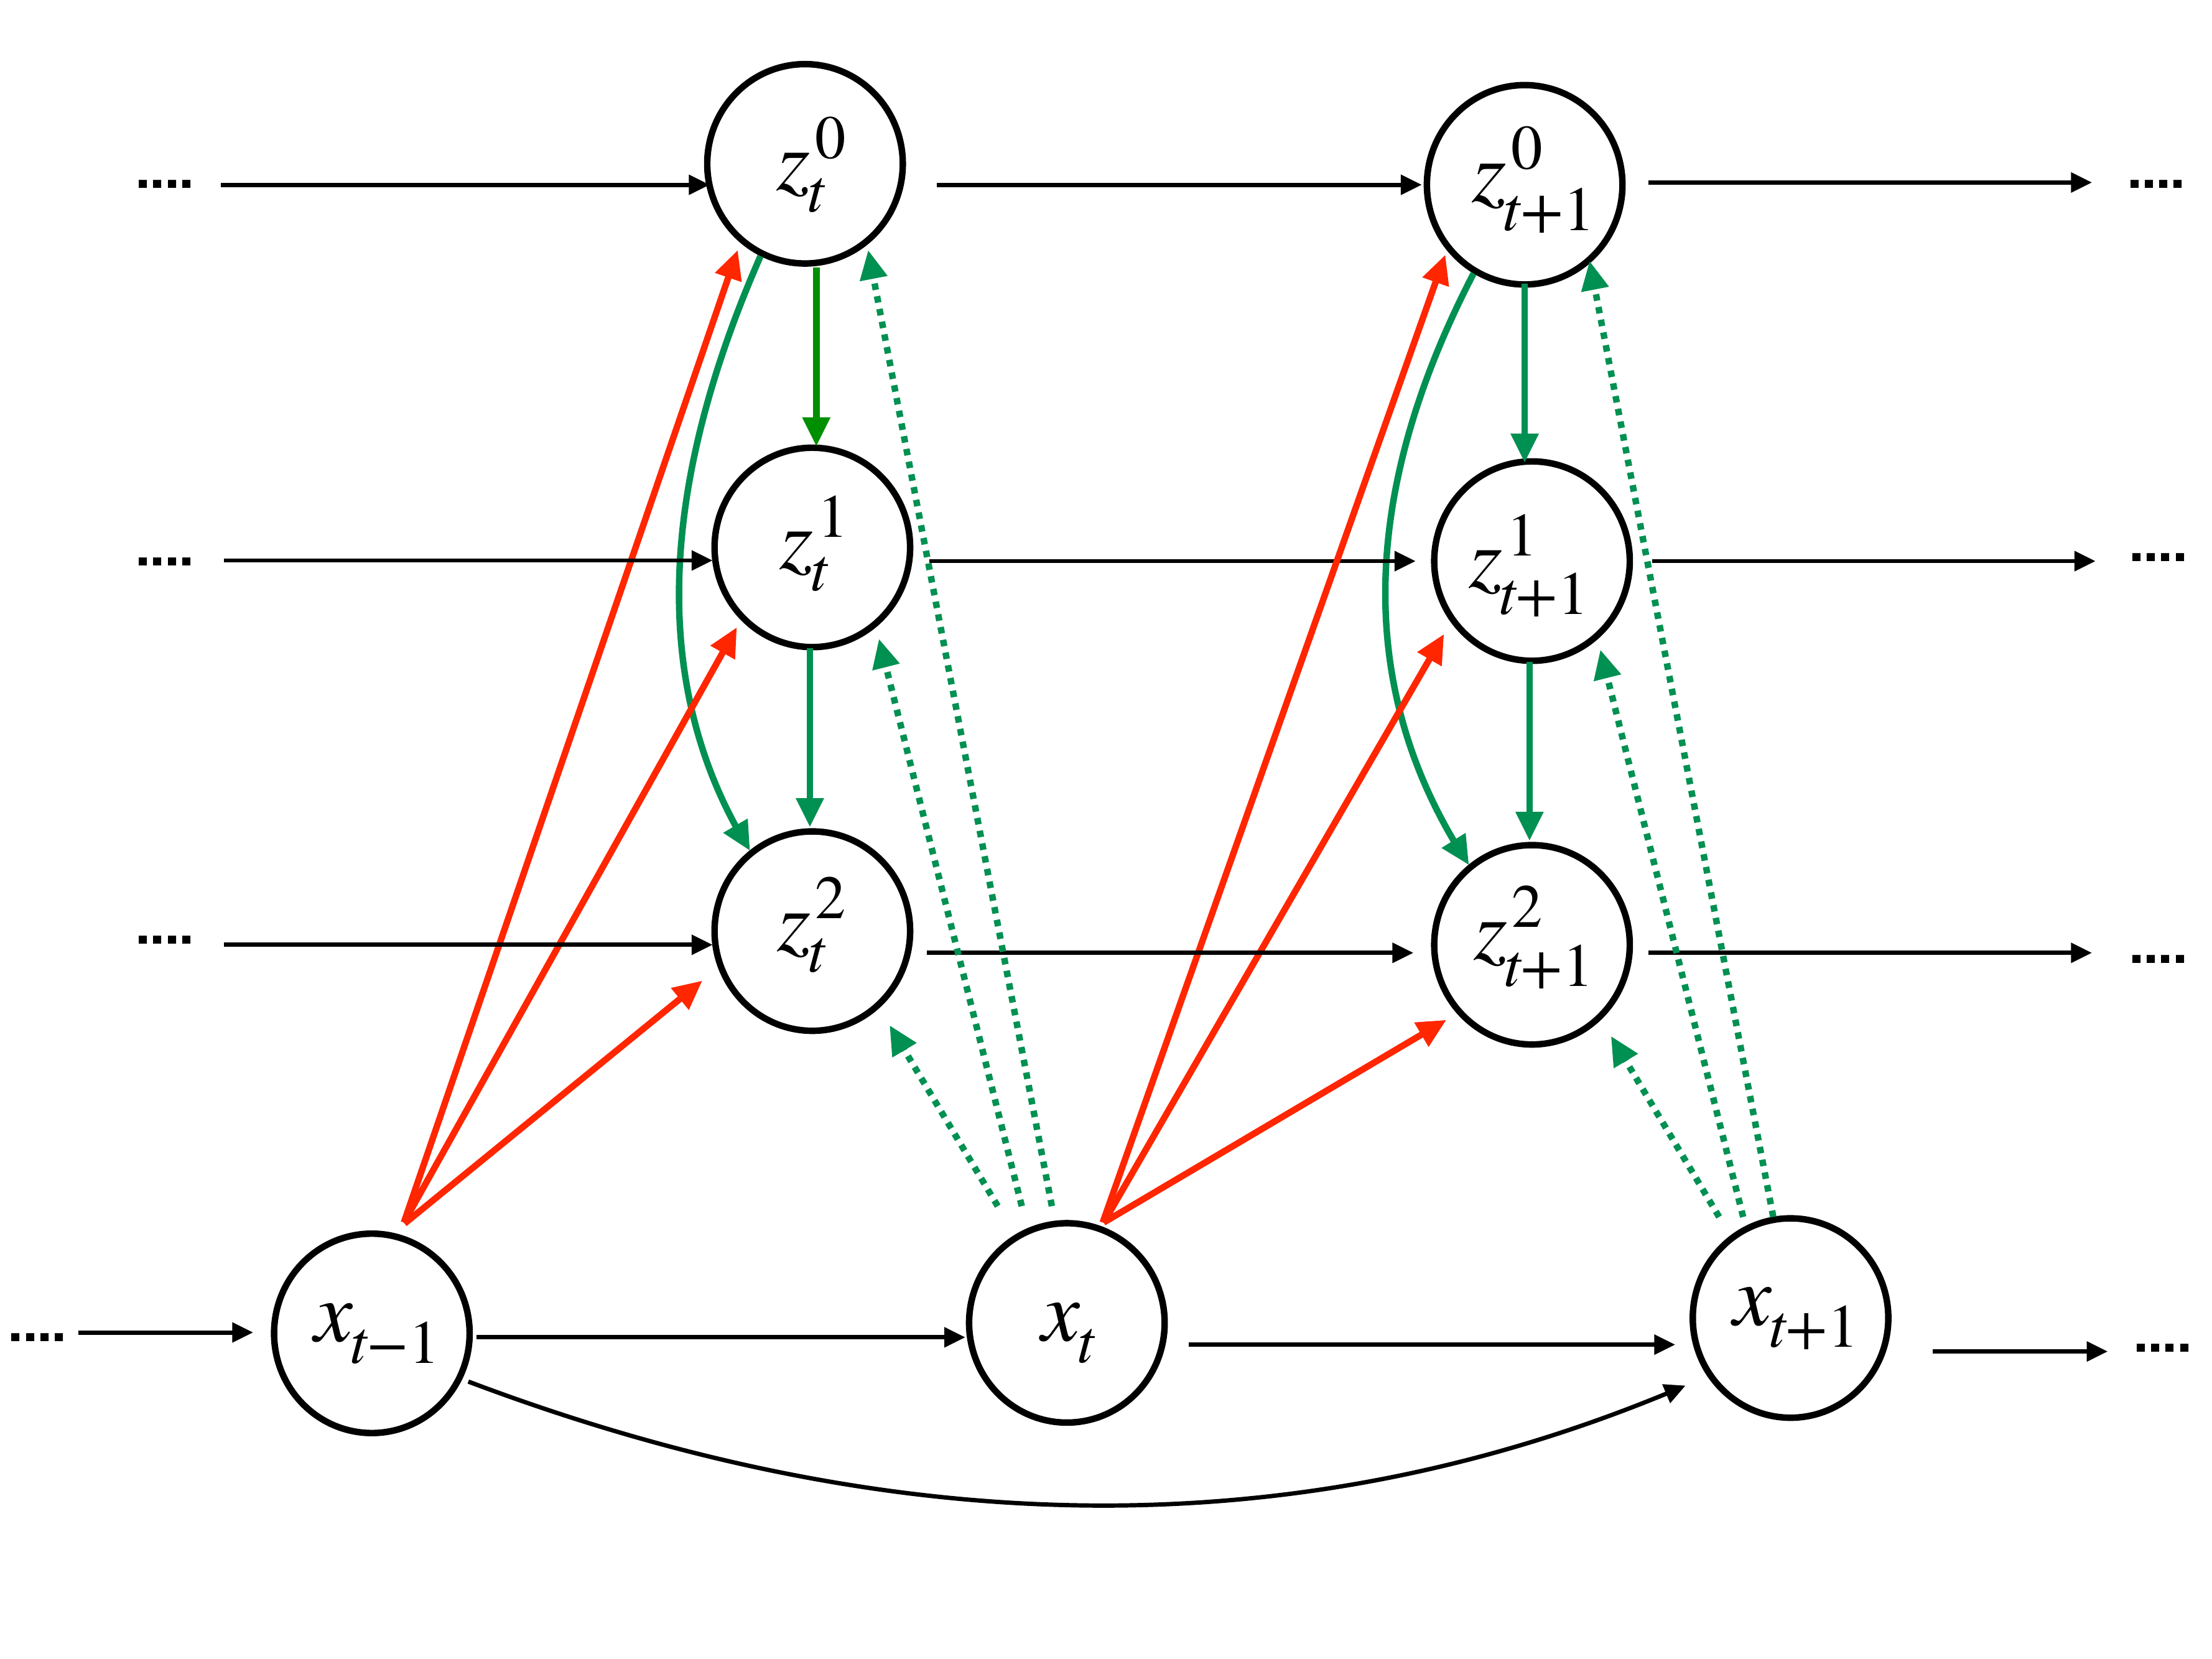}
 \end{center}
    \caption{\textbf{Schematic view of the approximate posterior with the dense-connectivity pattern}. Arrows in \textcolor{red}{red} show the connections from the input at the previous timestep to current latent variables. Arrows in \textcolor{green}{green} highlight skip connections between latent variables to outputs. Arrows in \textbf{black} indicate recurrent temporal connections. We empirically observe that this dense-connectivity pattern eases the training of latent hierarchy.}
    \label{fig:latent_model_inference}
\end{figure}

Fig~\ref{fig:latent_model_inference} illustrates the dense connection of the approximate posterior. For each latent variable has a deterministic connection to $x_{t-1}$ (red arrows in Fig~\ref{fig:latent_model}), in addition to all the latent variables from the layers below (green arrow in in Fig~\ref{fig:latent_model}). Finally , each latent variable has a direct connection to the output variables $x_{t}$, corresponding to the inference path.

\section{Additional Experimental Settings}

\subsection{Model Specification}
\label{app:model}

We specify the architecture used for the 64x64 model.
Convolutional layers in our model use 3x3 kernels with stride $s=1$ and padding $p=1$ unless otherwise specified.
We use modified Resnet blocks made up of two groups of ReLU + Conv2D + GroupNorm. 
GroupNorm layers use $g=16$ groups, except when operating on 1x1 tensors, in which case the only option is to use $g=1$.
Transposed Convolutions use 4x4 kernels with stride $s=2$ and padding $p=1$, which upscales 2x the input tensor.
ConvLSTM layers use 3x3 kernels with stride $s=1$ and padding $p=1$ and GroupNorm.
 
\begin{table}[h]
\centering
% [inline block 0: 14 envs, 183363 chars -> data_tex | \begin{tabular}{ccc} 	\toprule...]

    \caption{\textbf{Random Test Samples for Stochastic Moving MNIST.}}
\end{figure*}
\endgroup
