# Supplementary material for: Improved Conditional VRNNs for Video Prediction
Source: arXiv:1904.12165 source file (2019-04-27)
Supplement: Supplementary file 4 [file appendix_fig_samples_pushbair.tex]

\begingroup
\setlength{\tabcolsep}{0.5pt} %
\begin{figure*}[!t]
    \small
    \centering
    % [inline block 0: 4 envs, 70203 chars -> data_tex | \begin{tabular}{ccc|ccccccccccc}             &...]

    \caption{\textbf{Random Test Samples for pushbair.}}
\end{figure*}
\endgroup
